# Supplementary material for: Quantum Robustness Verification: A Hybrid Quantum-Classical Neural Network Certification Algorithm
Source: arXiv:2205.00900 source file (2022-08-12)
Supplement: Supplementary file 1 [file additional_material.tex]

In the first case, we access the hybrid solver from D-Wave Leap cloud, which embeds a part of the problem into the advantage system 5.1 constructed with 5760 qubits. In the second case, we used the QAOA runtime program of the IBMQ cloud on the IBM Brooklyn QC having the Hummingbird r2 architecture of 65 qubits and a quantum volume of 32.

\textbf{Solvers.}
We tested \textit{HQ-CRAN} with different solvers for the master problem of \autoref{eq:qubo}:
\begin{itemize}
    \itemsep-0.3em 
    \item Classic Computing
    \begin{enumerate}
        \item \textbf{Real}: IBM ILOG CPLEX\footnote{IBM (2020) IBM ILOG CPLEX 20.1 User’s Manual (IBM ILOG CPLEX Division, Incline Village, NV)} solver with real objective $p$ and real artificial variables. %\todo{should be better described?}
        \item \textbf{Anneal}: Simulated annealing\footnote{D-Wave-Neal 0.5.9 simulated annealing sampler.} algorithm. A Probabilistic technique for approximating the global optimum.
    \end{enumerate}
    \item Quantum Computing
    \begin{enumerate}
        \item \textbf{QAOA}: QAOA runtime algorithm implemented on gate-based quantum computer.
        \item \textbf{Leap}: D-Wave Leap hybrid algorithm which further decomposes and embeds the problem into a Quantum Annealing processing unit.
    \end{enumerate}
\end{itemize}

\begin{table*}[htbp]
\captionsetup{font=scriptsize}
\caption{Hybrid Benders decomposition applied to the robustness verification of neural networks. We use real variables for $p$ and $a_k$ and CPLEX to solve both master and sub problems. The maximum number of iterations has been set to $500$ and the gap to $1$. We run each algorithm on the first 100 samples of the MNIST dataset. The average time is per class.}
\begin{center}
\begin{footnotesize}
\begin{sc}
\begin{tabular}{lcccccccc|}
\toprule
\multirow{2}{*}{Networks} & \multirow{2}{*}{$\epsilon$} &\multicolumn{2}{c}{Optimality Ratio $\uparrow$} &\multicolumn{2}{c}{\# Iterations $\downarrow$} &\multicolumn{2}{c}{Time [sec.]} \\
&  &v1 &v2 &v1 &v2 &v1 &v2 \\
\midrule
\multirow{4}{*}{PGD-$2$x$[20]$} 
&$\nicefrac{1}{255}$ &$0.94\pm0.04$ &$0.94\pm0.04$     &$4\pm2$ &$3\pm1$           &$0.34$ &$0.31$ \\
&$\nicefrac{2}{255}$ &$0.93\pm0.05$ &$0.93\pm0.05$     &$6\pm2$ &$4\pm1$           &$0.52$ &$0.36$ \\
&$\nicefrac{4}{255}$ &$0.91\pm0.12$ &$0.92\pm0.08$     &$10\pm9$ &$6\pm18$         &$1.14$ &$0.61$ \\
&$\nicefrac{8}{255}$ &$0.85\pm0.56$ &$0.87\pm0.44$     &$27\pm25$ &$9\pm5$         &$4.26$ &$1.10$ \\
\midrule
\multirow{4}{*}{MLP-$2$x$[20]$} 
&$\nicefrac{1}{255}$ &$0.95\pm0.03$ &$0.95\pm0.03$      &$5\pm3$    &$4\pm2$        &$0.38$   &$0.33$  \\
&$\nicefrac{2}{255}$ &$0.94\pm0.04$ &$0.94\pm0.04$      &$8\pm5$    &$6\pm18$         &$0.64$  &$0.54$  \\
&$\nicefrac{4}{255}$ &$0.91\pm0.08$ &$0.92\pm0.07$      &$16\pm15$  &$8\pm5$          &$1.70$  &$0.72$  \\
&$\nicefrac{8}{255}$ &$0.83\pm0.45$ &$0.86\pm0.26$      &$58\pm60$  &$19\pm16$        &$14.50$ &$2.43$  \\
\bottomrule
\end{tabular}
\end{sc}
\end{footnotesize}
\label{tab:improvements}
\end{center}
\end{table*}
