# Supplementary material for: Quantum Robustness Verification: A Hybrid Quantum-Classical Neural Network Certification Algorithm
Source: arXiv:2205.00900 source file (2022-08-12)
Supplement: Supplementary file 2 [file appendix.tex]

\section{Matrices Construction} \label{app:matrix-construction}

Starting from the verification problem of a fully connected network with ReLU activation functions,
\begin{equation} \label{eq:general_verification_appendix}
\begin{aligned} 
    \min_{\vect{z}_i,\hat{\vect{z}}_i \in \mathbb{R}^{n_{i}}} &\left[\vect{z}_L\right]_c - \left[\vect{z}_L\right]_t \\
    \text{subject to} \quad  &\vect{z}_0\in \mathbb{B}^{p}_{\epsilon}(\vect{x}), \\
    &\hat{\vect{z}}_{i} = \matr{W}_i\vect{z}_{i - 1} + \vect{b}_i, \\
    &\vect{z}_i = \max\left\{0, \hat{\vect{z}}_i\right\}, \\ 
    &\forall i \in \left\{1,\dots,L\right\},
\end{aligned}
\end{equation}
we focus on the $p_\infty$-norm around $\vect{x}$ and we model the constraint $\vect{z}_0 \in \mathbb{B}^{\infty}_{\epsilon}(\vect{x})$ with two inequalities: $\vect{x} - \vect{z}_0 \leq \epsilon \cdot \vect{1}_{n_0}$ and $\vect{z}_0 - \vect{x} \leq \epsilon \cdot \vect{1}_{n_0}$. To deal with the activation functions, we propagate the boundaries through the network and model the ReLU units as \autoref{eq:complete_verification}. The initial boundaries are defined as $\bm{\ell}_0 = \vect{x} - \epsilon \cdot \vect{1}_{n_0}$ and $\vect{u}_0 = \vect{x} + \epsilon \cdot \vect{1}_{n_0}$. In our analysis, we rely on the interval arithmetic (IA) method to propagate the boundaries,
\begin{equation}\label{eq:interval_arithmetic}
    \begin{aligned}
        \bm{\ell}_i &= \matr{W}^-_i\vect{u}_{i-1} + \matr{W}^+_i\bm{\ell}_{i-1}, \\
        \vect{u}_i &= \matr{W}^+_i\vect{u}_{i-1} + \matr{W}^-_i\bm{\ell}_{i-1}, \\
        \matr{W}^+_i &= \max\left\{ \matr{W}_i, 0 \right\}, \\ 
        \matr{W}^-_i &= \min\left\{ \matr{W}_i, 0 \right\},
    \end{aligned}
\end{equation}
an efficient but over conservative method.
So, we can rewrite (\ref{eq:general_verification_appendix}) as
\begin{subequations}
\begin{align} \label{eq:complete_verification_appendix}
    \min_{\vect{z}_i \in \mathbb{R}^{n_{i}}} &\left[\vect{z}_L\right]_c - \left[\vect{z}_L\right]_t \\
    \text{subject to} \quad  &\vect{x} - \vect{z}_0 \leq \epsilon, \\
    &\vect{z}_0 - \vect{x} \leq \epsilon,  \\
    &\vect{z}_i \leq \matr{W}_i\vect{z}_{i - 1} + \vect{b}_i - \bm{\ell}_i \odot \left(\vect{1}_{n_i}-\vect{y}_i\right), \label{eq:constraint_bounds_1_app} \\
    &\vect{z}_i \leq \vect{u}_i \odot \vect{y}_i, \label{eq:constraint_bounds_2_app}\\
    &\vect{z}_i \geq \matr{W}_i\vect{z}_{i - 1} + \vect{b}_i, \\
    &\vect{z}_i \geq \vect{0}_{n_i}, \\
    &\vect{y}_i \in \left\{0,1\right\}^{n_i}, \quad \forall i \in \left\{1,\dots,L\right\},
\end{align}
\end{subequations}
where we encapsulate $\vect{z}_i = \matr{W}_i\hat{\vect{z}}_{i-1} + \vect{b}_i$ within the inequalities. In the same way as \citet{tjeng2018evaluating},
if we only consider \textit{unstable} neurons we can get rid of some constraints. A neuron $j$ of layer $i$ is \textit{stable inactive} if its upper bound $[\vect{u}_i]_j$ is $\leq 0$, so we can constrain $[\vect{y}_i]_j$ to be zero. This will lead to the following logic $[\vect{z}_i]_j \leq [\matr{W}_i\vect{z}_{i - 1}]_j + [\vect{b}_i]_j - [\bm{\ell}_i]_j$ for \autoref{eq:constraint_bounds_1_app} and $[\vect{z}_i]_j \leq 0$ for \autoref{eq:constraint_bounds_2_app}. Similarly, a neuron is \textit{stable active} if its lower bound $[\bm{\ell}_i]_j$ is $\geq 0$ and we can constrain $[\vect{y}_i]_j$ to be one, leading to $[\vect{z}_i]_j \leq [\matr{W}_i\vect{z}_{i - 1}]_j + [\vect{b}_i]_j$ for \autoref{eq:constraint_bounds_1_app} and $[\vect{z}_i]_j \leq [\vect{u}_i]_j$ for \autoref{eq:constraint_bounds_2_app}. Indeed, a neuron is $unstable$ when its boundaries are $[\bm{\ell}_i]_j \leq 0$ and $[\vect{u}_i]_j \geq 0$. We further arrange \autoref{eq:complete_verification_appendix} to
\begin{equation} \label{eq:complete_verification_arrenged_appendix}
\begin{aligned} 
    \min_{\vect{z}_i \in \mathbb{R}^{n_{i}}} &\left[\vect{z}_L\right]_c - \left[\vect{z}_L\right]_t \\
    \text{subject to} \quad  &\vect{z}_0 \geq \bm{\ell}_0, \\
    & - \vect{z}_0 \geq - \vect{u}_0,  \\
    &\matr{W}_i\vect{z}_{i - 1} - \vect{z}_i + \bm{\ell}_i \odot \vect{y}_i \geq \bm{\ell}_i -\vect{b}_i,  \\
    &- \vect{z}_i + \vect{u}_i\odot \vect{y}_i \geq 0,  \\
    &- \matr{W}_i\vect{z}_{i - 1} + \vect{z}_i \geq \vect{b}_i, \\
    &\vect{z}_i \geq 0, \\
    &\vect{y}_i \in \left\{0,1\right\}^{n_i}, \quad \forall i \in \left\{1,\dots,L\right\},
\end{aligned}
\end{equation}
where we shift the inequalities so that they match in sign. Let us define $n_z = n_0 + \dots + n_L$ equal to the total number of neurons and $n_y$ equal to the number of \textit{unstable} neurons. $\vect{z} \in \mathbb{R}^{n_z}$ is a vector composed by all logits $\left(\vect{z}_0, \vect{z}_1, \dots, \vect{z}_L \right)$ and $\vect{y} \in \left\{0, 1\right\}^{n_y}$ is a vector of binary variables which model the \textit{unstable} neurons. Furthermore, we define $\bm{\ell}, \bm{u} \in \mathbb{R}^{n_z}$, as vectors of lower and upper bounds for all neurons and $\tilde{\bm{\ell}} \in \mathbb{R}^{n_y}$, as vector of lower bounds only for \textit{unstable} neurons. Similarly, we define $\bar{\vect{b}}$ equal to the biases of all neurons and $\tilde{\vect{b}}$ equal to the biases of only the \textit{unstable} neurons. We can now define the following matrices:
%
% \begin{equation*}
% \matr{M} =
% \left[\begin{array}{ccccc}
%     -\matr{W}_1 & \matr{I}_{n_1} & \matr{O}_{n_1 \times n_2} & \cdots & \matr{O}_{n_1 \times n_L} \\
%     \matr{O}_{n_2 \times n_0} & -\matr{W}_2 & \matr{I}_{n_2} & \cdots & \matr{O}_{n_2 \times n_L} \\
%     \vdots & & \ddots & \ddots & \vdots \\
%     \matr{O}_{n_L \times n_0} & \dots &  \dots & -\matr{W}_L & \matr{I}_{n_L}
% \end{array}\right],
% \end{equation*}
% \begin{equation*}
% \matr{N} =
% \left[\begin{array}{cccc}
%     \matr{O}_{n_1 \times n_0} & \matr{I}_{n_1} & \cdots & \matr{O}_{n_1 \times n_L} \\
%     \vdots & & \ddots & \vdots \\
%     \matr{O}_{n_L \times n_0} & \cdots & \cdots & \matr{I}_{n_L} 
% \end{array}\right],
% \end{equation*}
% %
% \begin{equation*}
% \hat{\matr{C}} = 
% \left[\begin{array}{cc}
%     \matr{I}_{n_0} & \matr{O}_{n_0 \times \left(n_1 + \dots + n_L \right)} \\
%     -\matr{I}_{n_0} & \matr{O}_{n_0 \times \left(n_1 + \dots + n_L \right)} 
% \end{array}\right],
% \end{equation*}
% \begin{equation*}
% \matr{C} = 
% \left[\begin{array}{c}
%     \hat{\matr{C}} \\
%     \matr{M} \\
%     \matr{N}        
% \end{array}\right], 
% \end{equation*}
\begin{equation*}
\matr{L} = \texttt{diag} (\tilde{\bm{\ell}}), \quad
\matr{U} = \texttt{diag} \left(\vect{u} \right),
\end{equation*}
\begin{equation*}
\matr{A} = 
\left[\begin{array}{c}
    \hat{\matr{A}} \\
    - \matr{N}
\end{array}\right], \quad 
\text{where} \quad
\hat{\matr{A}}_{j :} =
\left\{
\begin{aligned}
    \matr{O}_{1 \times n_z} \quad &\text{if} \, [\vect{u}]_j \leq 0, \\
    -\matr{M}_{j:} \quad &\text{otherwise,}
\end{aligned}
\right.
\end{equation*}
\begin{equation*}
\matr{B} =
\left[\begin{array}{c}
\matr{L} \\
\hat{\matr{B}}
\end{array}\right], \quad 
\text{where} \quad
\hat{\matr{B}}_{j:} = \left\{
\begin{aligned}
    &\matr{U}_{j:} \quad \text{if} \; [\bm{\ell}]_j \leq 0 \, \text{and} \, [\vect{u}]_j \geq 0, \\
    &\matr{O}_{1 \times n_y} \quad \text{otherwise,}
\end{aligned}\right.
\end{equation*}
\begin{equation*}
\text{and the following vectors:} \quad
\vect{b} = 
\begin{pmatrix}
\tilde{\vect{b}} - \tilde{\bm{l}} \\ 
\hat{\vect{b}}
\end{pmatrix}, 
\end{equation*}
\begin{equation*}
[\hat{\vect{b}}]_j = 
\left\{\begin{aligned}
    &-[\vect{u}]_j \quad \text{if} \; [\bm{\ell}]_j \geq 0, \\
    &0 \quad \quad \text{otherwise,}
\end{aligned}\right. 
\quad \text{and} \quad
\vect{d} = 
\begin{pmatrix}
\bm{\ell}_0 \\
- \vect{u}_0 \\ 
\bar{\vect{b}} \\ 
\vect{0}
\end{pmatrix}.
\end{equation*}
At this point, we can write \autoref{eq:complete_verification_arrenged_appendix} in a concise matrix formulation as:
\begin{equation*}
\begin{aligned}
&\min_{\vect{z} \in \mathbb{R}^{n_z},\vect{y} \in \left\{0, 1\right\}^{n_y}} &\quad&\vect{g}^{\intercal}\vect{z} \\
    &\qquad\,\,\,\text{subject to} &&\matr{A}\vect{z} + \matr{B}\vect{y} \geq \vect{b} \\
    &&&\matr{C}\vect{z} \geq \vect{d}
\end{aligned}
\end{equation*}
where $\vect{g} \in \mathbb{R}^{n_z}$ is a vector of zeros having $1$ at $[\vect{z}]_c$ position and $-1$ at $[\vect{z}]_t$ of $\vect{z}$, respectively.
